# Supplementary material for: Effect of the charged-lepton's mass on the quasielastic neutrino cross sections
Source: arXiv:1707.01014 ancillary file (2017-09-07)
Supplement: Supplementary file 1 [file SupplementalMaterial.pdf]

# Effect of the charged-lepton's mass on the quasielastic neutrino cross sections. Supplemental Material

Artur M. Ankowski*
*Center for Neutrino Physics, Virginia Tech, Blacksburg, Virginia 24061, USA*

To give a deeper insight into the behavior of the $\frac{d\sigma(\nu_\mu)}{d\cos\theta}/\frac{d\sigma(\nu_e)}{d\cos\theta}$ ratios discussed in this article, in Figs. 1 and 2, I present the double differential cross sections $d\sigma/d\omega d\Omega$ for charged-current quasielastic scattering off carbon.

Figure 1 shows the results calculated within the relativistic Fermi gas model for the scattering angles 5 and 60 degrees and the neutrino energies 200 and 600 MeV. When the effect of Pauli blocking is taken into account, the single differential cross section $d\sigma/d\cos\theta$ for scattering at 5 degrees is higher for muon neutrinos than for electron neutrinos. Although within the kinematically allowed $\omega$ range for $\nu_e$ scattering and not too close to its boundaries, the cross section $d\sigma/d\omega d\Omega$ for electron neutrinos is higher than that for muon neutrinos, the allowed $\omega$ ranges are broader for muon neutrinos than for electron neutrinos, yielding the higher integrated $\nu_\mu$ results. On the other hand, when the allowed $\omega$ ranges are not constrained by Pauli blocking, the cross section for electron neutrinos is not suppressed and turns out to be higher than for muon neutrinos.

In the spectral function approach, the allowed $\omega$ ranges extend to the values low enough that the suppression of the cross sections for electron neutrinos does not appear, and the integrated results are higher than that for muon neutrinos, see Fig. 2. This conclusion holds true also when only the mean-field (shell-model) part of the spectral function is employed in the calculations, because of the small correlated contribution to the cross sections at the discussed kinematics.

Among the considered descriptions of the carbon nucleus, only the relativistic Fermi gas model with Pauli blocking predicts at some kinematics the cross section $d\sigma/d\cos\theta$ to be higher for muon neutrinos than for electron neutrinos, and this feature appears solely at small scattering angles and sufficiently high neutrino energy. I illustrate these findings in Figs. 3 and 4, presenting the results for the neutrino energies 140 MeV, 170 MeV, 200 MeV, and 600 MeV, obtained within the relativistic Fermi gas model with and without Pauli blocking, and within the spectral function approach employing the full spectral function or only its mean-field part.

As a final remark, I would like to note that in the approach of Ref. [1], final-state interactions do not affect the single differential cross sections $d\sigma/d\cos\theta$, discussed in this article. However, one needs to keep in mind that at low energies and small scattering angles, they significantly affect the double differential cross sections $d\sigma/d\omega d\Omega$, but were not accounted here.

* ankowski@vt.edu

[1] A. M. Ankowski, O. Benhar, and M. Sakuda, Phys. Rev. D **91**, 033005 (2015)

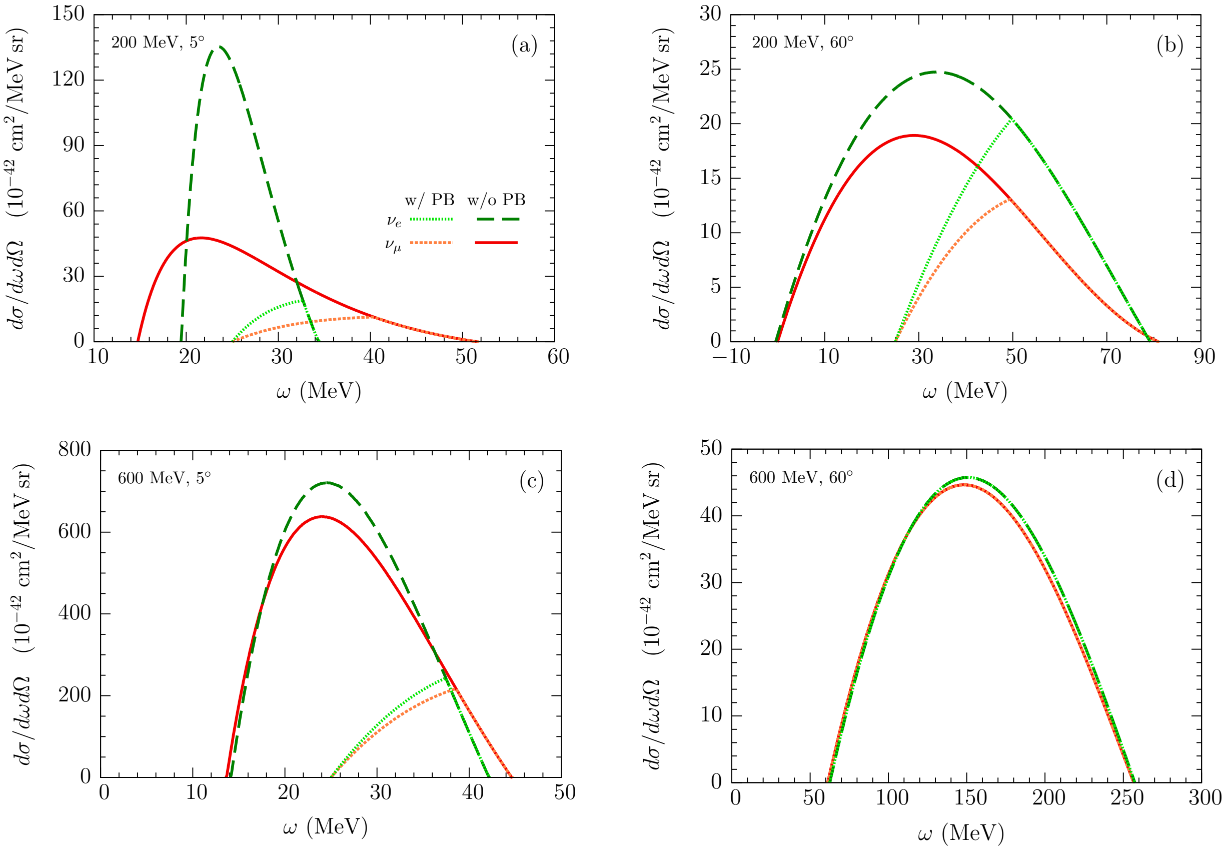


FIG. 1. Double differential cross sections $d\sigma/d\omega d\Omega$ for charged-current quasielastic scattering of electron and muon neutrinos off carbon, calculated within the relativistic Fermi gas model with and without Pauli blocking at different neutrino energies and scattering angles. Note that in panel (d), Pauli blocking does not play any role and the results with and without this effect coincide.

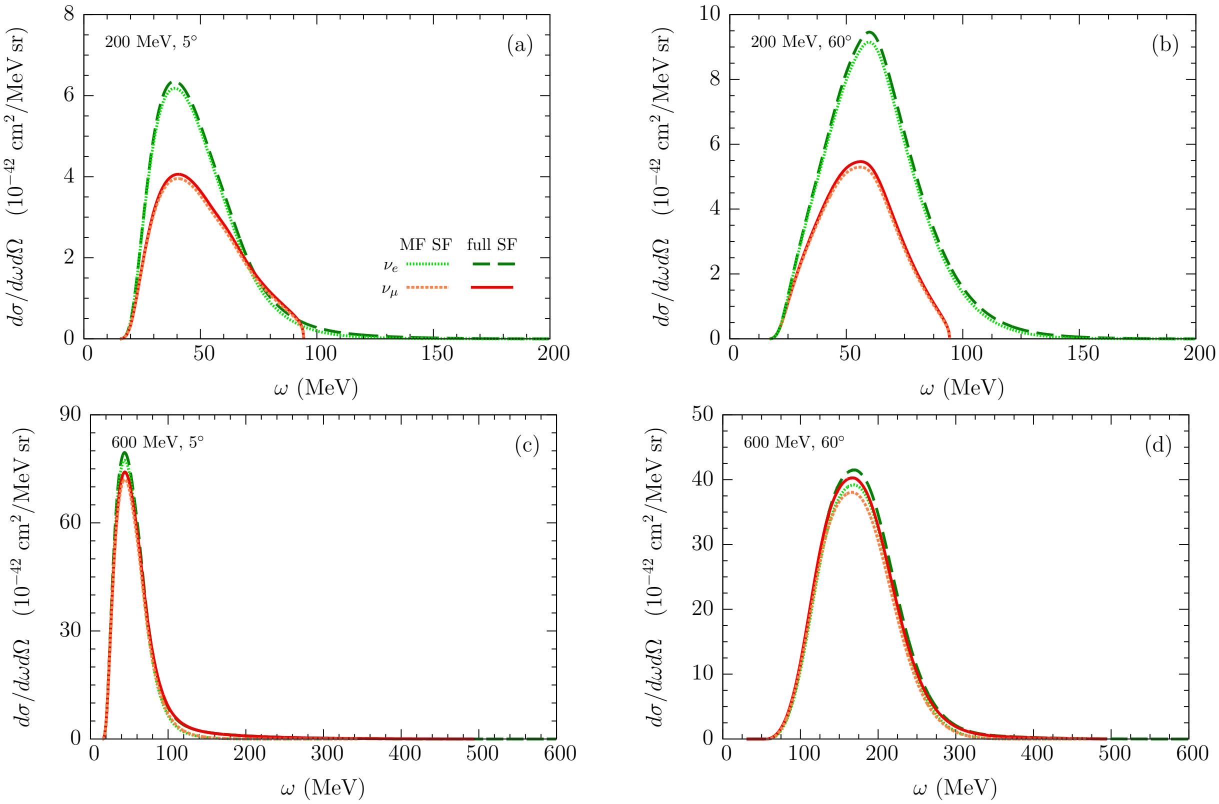


FIG. 2. Same as Fig. 1 but for carbon nucleus described using the mean-field part and full spectral function.

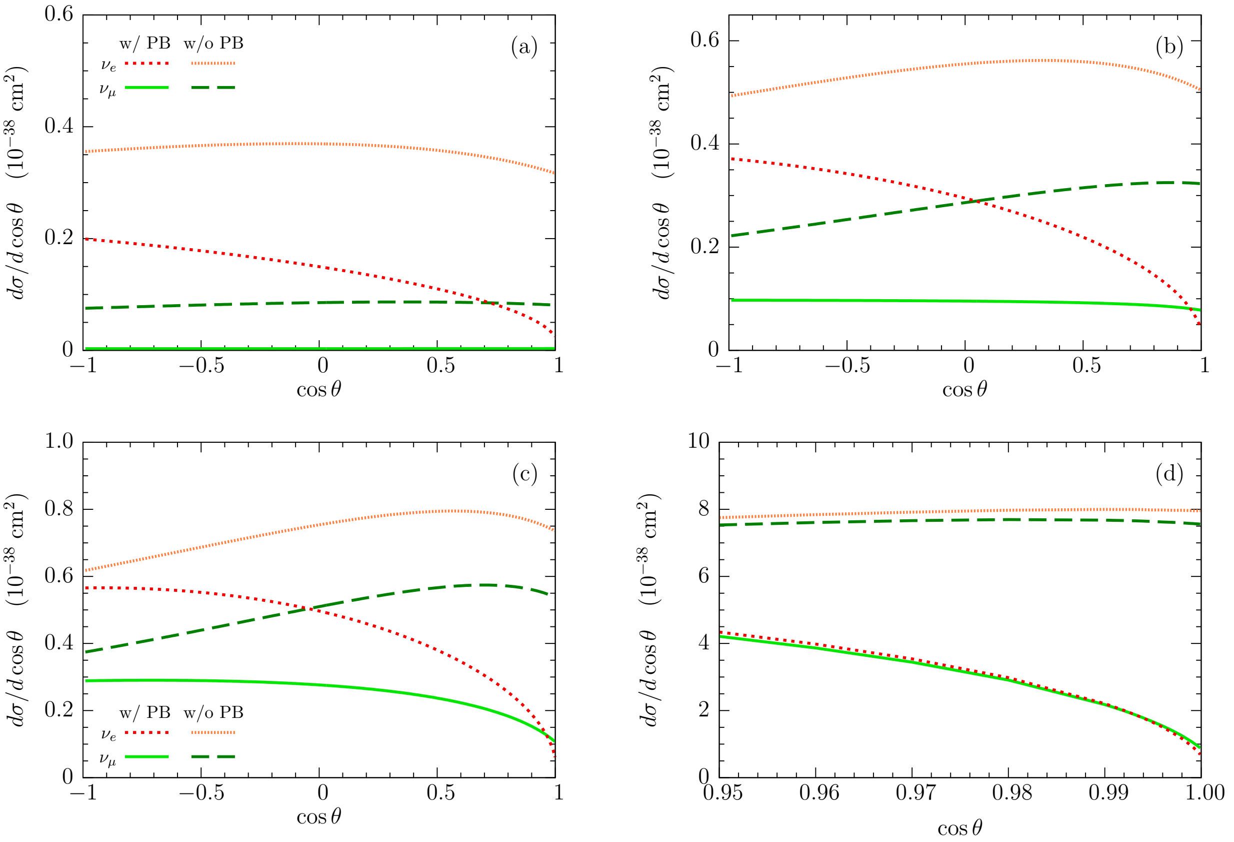


FIG. 3. Differential cross sections $d\sigma/d\cos\theta$ for charged-current quasielastic scattering of electron and muon neutrinos off carbon, calculated within the relativistic Fermi gas model with and without Pauli blocking at neutrino energies (a) 140 MeV, (b) 170 MeV, (c) 200 MeV, and (d) 600 MeV. Note that in panel (d), zero is suppressed in the $x$ axis.

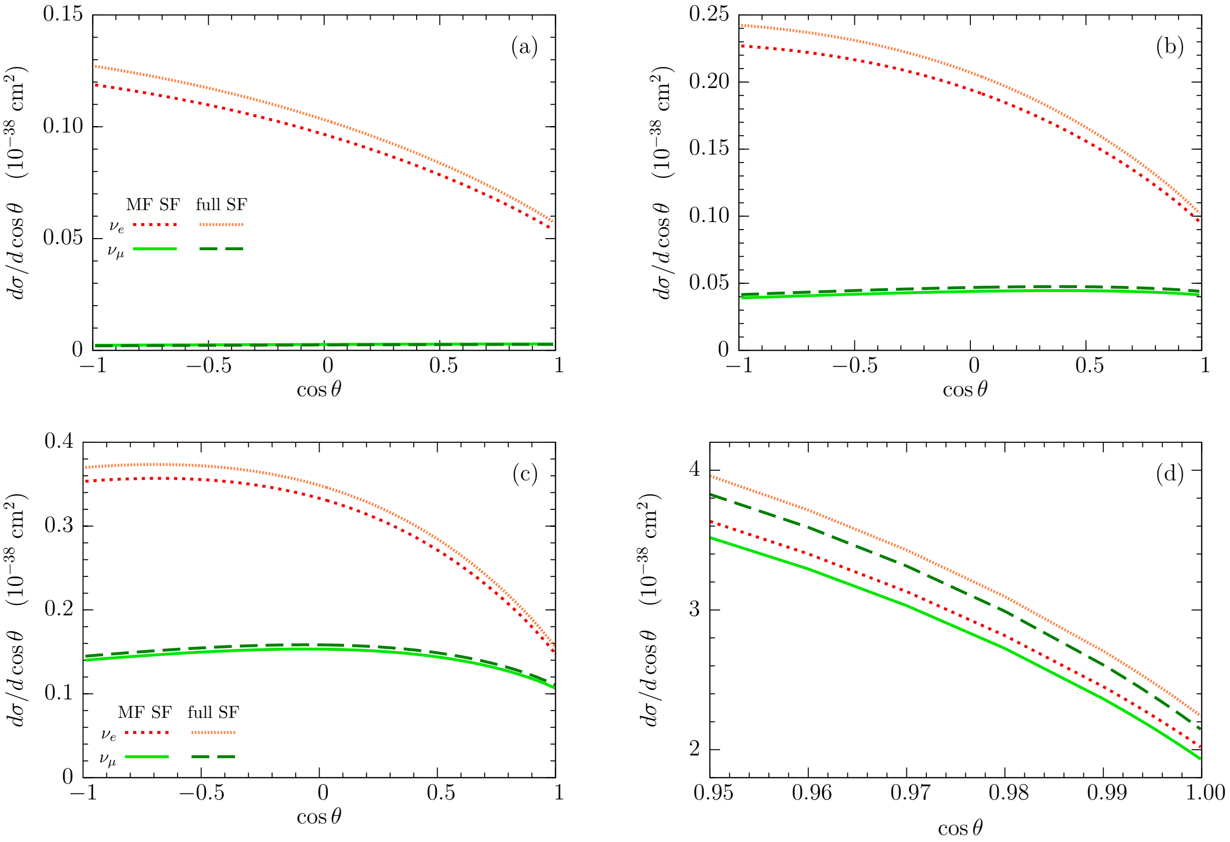


FIG. 4. Differential cross sections $d\sigma/d\cos\theta$ for charged-current quasielastic scattering of electron and muon neutrinos off carbon, calculated using the mean-field part and full spectral function, at neutrino energies (a) 140 MeV, (b) 170 MeV, (c) 200 MeV, and (d) 600 MeV. Note that in panel (d), zero is suppressed in the $x$ and $y$ axes.
